# Supplementary material for: On the Batch Size Selection in Stochastic Gradient Methods Using No-Replacement Sampling
Source: arXiv:2506.08758 source file (2025-06-10)
Supplement: Supplementary file 1 [file appendix.tex]

\begin{appendices} \label{appendix_label}
Proof of proposition \ref{prop1}
\begin{proof} By using the sampling measure above introduced, we can write
$$
E[\nabla_{S_{\jmath}} f(x)] = \sum_{j=1}^{N_B}\frac{1}{N_B}\nabla_{S_{j}} f(x) = \sum_{j=1}^{N_B}\frac{1}{N_B}\frac{1}{N_S}\sum_{i\in S_j} \nabla f_i(x).
$$
Since $N_B=N/N_S$, it is obtained that
$$
E[\nabla_{S_{\jmath}} f(x)] = \frac{1}{N}\sum_{j=1}^{N_B}\sum_{i\in S_j} \nabla f_i(x) = \nabla f(x).
$$
For the variance $Var[\nabla_{S_{\jmath}} f(x)] = E[\|\nabla_{S_{\jmath}} f(x)-\nabla_ f(x)\|^2]$ we can write
\begin{align*}
    & E[\|\nabla_{S_{\jmath}} f(x)-\nabla_ f(x)\|^2] = E\left[\Big\Vert \frac{1}{N_S}\sum_{i\in S_\jmath} \nabla f_i(x) - \nabla f(x) \Big\Vert^2\right]\\
    =&E\left[\Big\Vert \frac{1}{N_S}\sum_{i\in S_\jmath} \Bigl(\nabla f_i(x) - \nabla f(x)\Bigr) \Big\Vert^2\right] = 
    E\left[ \frac{1}{N_S^2}\sum_{i\in S_\jmath} \|\nabla f_i(x) - \nabla f(x)\|^2 \right]\\
    &\quad+E\left[\frac{1}{N_S^2}\sum_{i\neq h\in S_\jmath} (\nabla f_i(x) - \nabla f(x))^T(\nabla f_h(x) - \nabla f(x)) \right].
\end{align*}
For the first term we can write
\begin{align*}
    &\frac{1}{N_B}\sum_{j=1}^{N_B}\frac{1}{N_S^2}\sum_{i\in S_j} \| \nabla f_i(x)-\nabla f(x)\|^2\\
    =&\frac{1}{N_S}\frac{1}{N}\sum_{j=1}^{N_B}\sum_{i\in S_j} \| \nabla f_i(x)-\nabla f(x)\|^2 = \frac{Var[\nabla f_{\imath}(x)]}{N_S}.
\end{align*}
For the second term we have 
\begin{align*}
&\frac{1}{N_B}\sum_{j=1}^{N_B}\frac{1}{N_S^2}\sum_{i\neq h\in S_\jmath} (\nabla f_i(x) - \nabla f(x))^T(\nabla f_h(x) - \nabla f(x))\\
&\frac{1}{N_S^2 N_B}\sum_{j=1}^{N_B}\sum_{i\neq h\in S_\jmath} (\nabla f_i(x) - \nabla f(x))^T(\nabla f_h(x) - \nabla f(x)).
\end{align*}
For any $j$, the inner sum has $2 {N_s\choose 2}$ terms, and determines the covariance $Cov_{S_j}[\nabla f_{i_j}(x),\nabla f_{h_j}(x)]$ of the items within batch $S_j$, i.e.
$$
Cov_{S_j}[\nabla f_{i_j}(x),\nabla f_{h_j}(x)]=\frac{1}{2{N_s\choose 2}}\sum_{{i_j}\neq {h_j}\in S_\jmath} (\nabla f_{i_j}(x) - \nabla f(x))^T(\nabla f_{h_j}(x) - \nabla f(x)),
$$
so that
$$
Cov[\nabla f_\imath(x),\nabla f_\jmath(x)] =\frac{1}{N_B}\sum_{\ell=1}^{N_B} Cov_{S_\ell}[\nabla f_{i_\ell}(x),\nabla f_{h_\ell}(x)]
$$
is the \textit{average batch covariance} of the component gradients. Then we can write
\begin{equation}
Var[\nabla_{S_{\jmath}} f(x)]=
    \frac{Var[\nabla f_{\imath}(x)]}{N_S} + \frac{1}{N_s^2}{2{N_s\choose 2}}\,Cov[\nabla f_\imath(x),\nabla f_\jmath(x)]. 
    \label{bcovar}
\end{equation}
Now, if $N_S=N$ it follows that  $Var[\nabla_{S_{\jmath}} f(x)]=0$, so that
$$
0 = \frac{Var[\nabla f_{\imath}(x)]}{N} + \frac{1}{N^2}{2{N\choose 2}}\,Cov[\nabla f_\imath(x),\nabla f_\jmath(x)],
$$
from which
$$
Cov[\nabla f_\imath(x),\nabla f_\jmath(x)] = -\frac{Var[\nabla f_{\imath}(x)]}{N-1}.
$$
By taking into account (\ref{bcovar}), we finally obtain that
\begin{align*}
    Var[\nabla_{S_{\jmath}} f(x)] =& \frac{Var[\nabla f_{\imath}(x)]}{N_S} - \frac{N_S-1}{N_S}\frac{Var[\nabla f_{\imath}(x)]}{N-1}\\
    =&\frac{Var[\nabla f_{\imath}(x)]}{N_S}\frac{N-N_S}{N-1}.
\end{align*}
\hfill\qed
\end{proof}

Proof of proposition \ref{prop2}

\begin{proof}
    
\begin{align*}
    &Var[\nabla f_{\imath}(x)]=\frac{1}{N}\sum_{i=1}^N\|\nabla f_{i}(x)-\nabla f(x)\|^2 \\&=\frac{1}{N}\sum_{j=1}^{N_B}\sum_{i\in S_j}\|\nabla f_{i}(x)-\nabla_{S_j} f(x)\|^2 + \frac{1}{N}\sum_{j=1}^{N_B}\sum_{i\in S_j}\|\nabla_{S_j} f(x)-\nabla f(x)\|^2\\
    \end{align*}
    where the mixed terms are omitted because are zero by construction. Therefore
    \begin{align}
    Var[\nabla f_{\imath}(x)]=&\frac{1}{N}\sum_{j=1}^{N_B}\sum_{i\in S_j}\|\nabla f_{i}(x)-\nabla_{S_j} f(x)\|^2 +\nonumber\\
    &\qquad \frac{1}{N}\sum_{j=1}^{N_B}N_S\|\nabla_{S_j} f(x)-\nabla f(x)\|^2\nonumber\\
    &=\frac{1}{N_B}\sum_{j=1}^{N_B}\frac{1}{N_S}\sum_{i\in S_j}\|\nabla f_{i}(x)-\nabla_{S_j} f(x)\|^2 +\nonumber\\
    &\qquad \frac{1}{N_B}\sum_{j=1}^{N_B}\|\nabla_{S_j} f(x)-\nabla f(x)\|^2 = W(x)+B(x).
\end{align}
\end{proof}

\end{appendices}
